# Supplementary material for: High-resolution Emission Spectroscopy of the Ultrahot Jupiter KELT-9b: Little Variation in Day- and Nightside Emission Line Contrasts
Source: arXiv:2304.03248 source file (2023-04-06)

Night 2

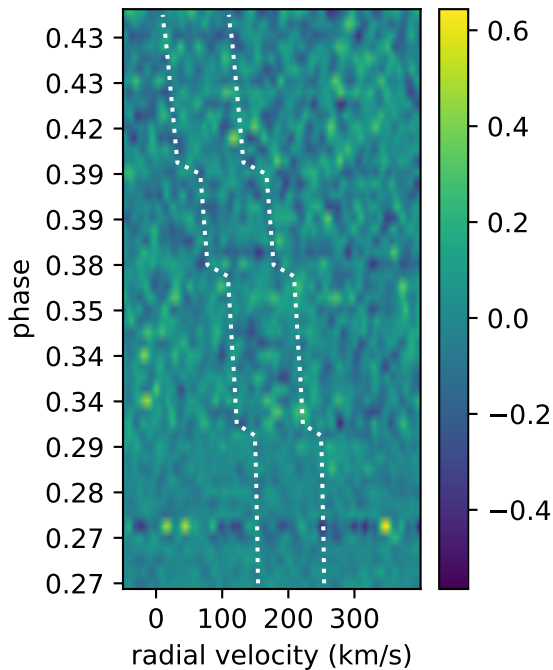

Night 3

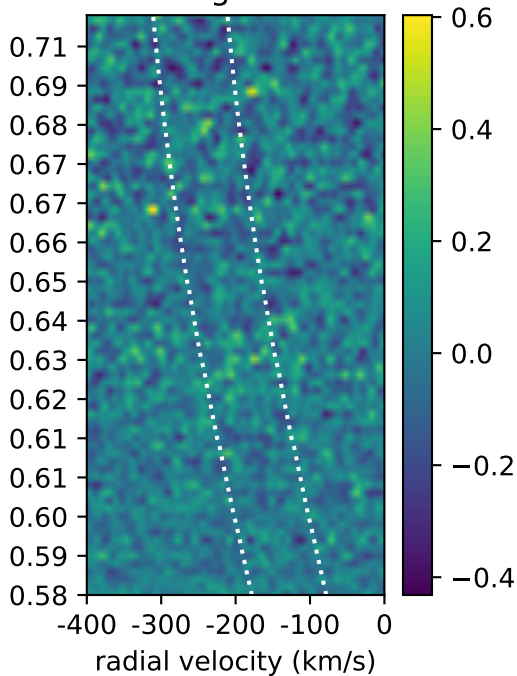

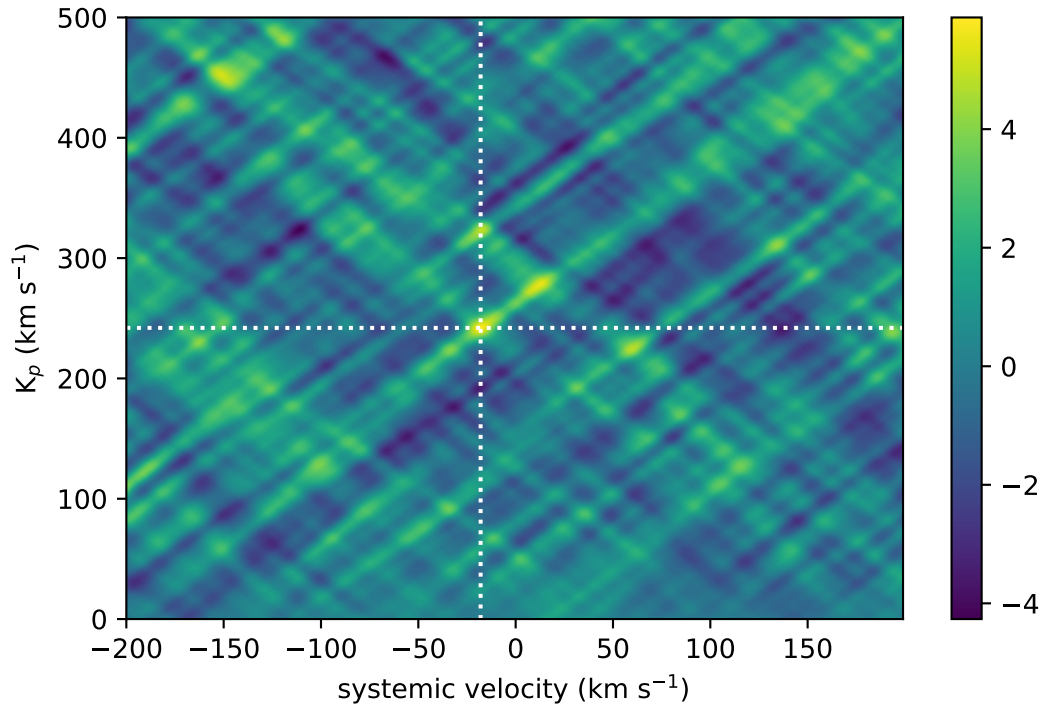

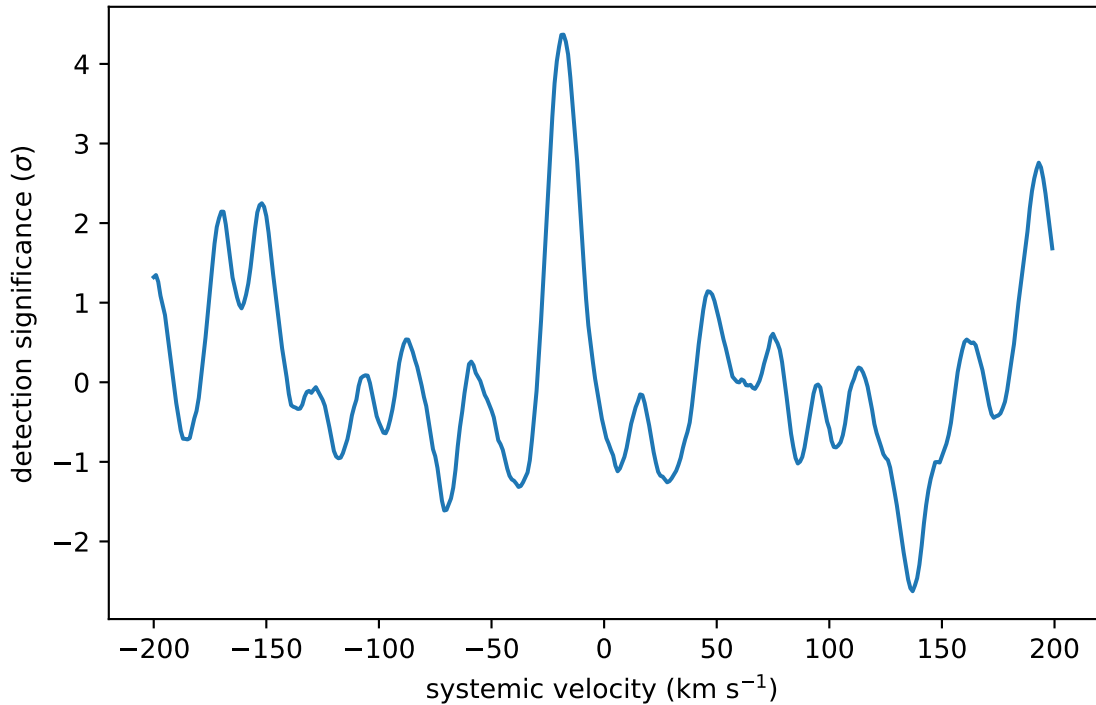

Supplement: Supplementary file 1 [file Si_Fossati2021_Solar_for_paper.pdf]
